# Supplementary material for: Noise-enabled goal attainment in crowded collectives
Source: arXiv:2507.08100 source file (2026-02-24)

a)

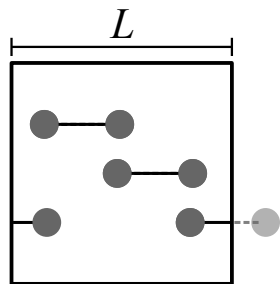

b)

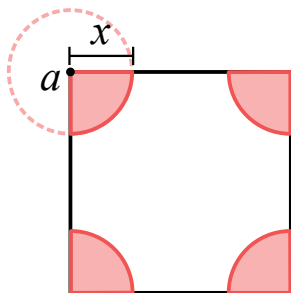

c)

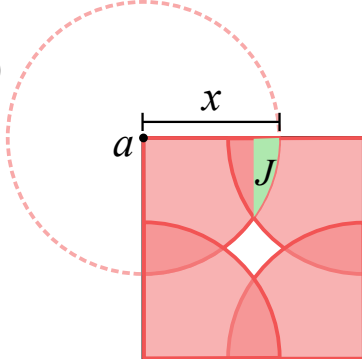

d)

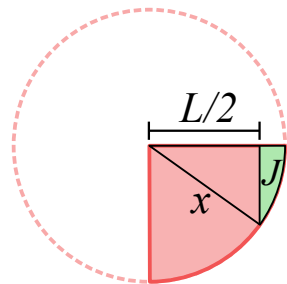

e)

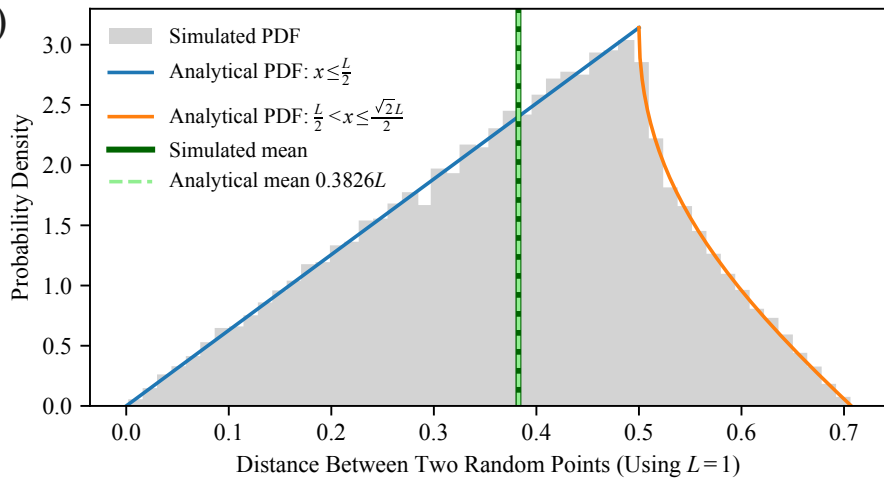

Supplement: Supplementary file 1 [file fig_si_torus_distances.pdf]
